# Supplementary material for: DocMSU: A Comprehensive Benchmark for Document-level Multimodal Sarcasm Understanding
Source: arXiv:2312.16023 source file (2023-12-26)
Supplement: Supplementary file 1 [file appendices.tex]

\documentclass[twocolumn]{article}
\usepackage{geometry}
\geometry{letterpaper,scale=0.8}
\usepackage[hidelinks]{hyperref}
\usepackage{newfloat}
\usepackage{listings}
\usepackage{bibentry}
\usepackage{graphicx}
\usepackage{wrapfig}
\usepackage{setspace}
\usepackage{float}

\usepackage{algorithm}
\usepackage{algpseudocode} 
\usepackage{tabularx}% NEW ADDED
\usepackage{multirow}% NEW ADDED
\usepackage{amsmath}% NEW ADDED
\usepackage{tabularray}% NEW ADDED
\usepackage{array}% NEW ADDED
\usepackage{booktabs}% NEW ADDED
\usepackage{subfigure}% NEW ADDED

\title{Supplementary Material for\\
DocMSU: A Comprehensive Benchmark for Document-level \\Multimodal Sarcasm Understanding}
\author{
Anonymous Submission
}
\date{}
\begin{document}
\maketitle
%\tableofcontents

%\section{Model Details}

%\appendix
\section{DocMSU Annotation Pipeline}

\subsection{Details of annotators}

There are $15$ undergraduate and postgraduate volunteers who participated in the work, and we report the annotators' education backgrounds and genders in Figure \ref{fig:annotator detail}. 
The age of these annotators ranges from 20 to 30.
\begin{figure}[h!]
    \centering
    \includegraphics[width=0.9\linewidth]{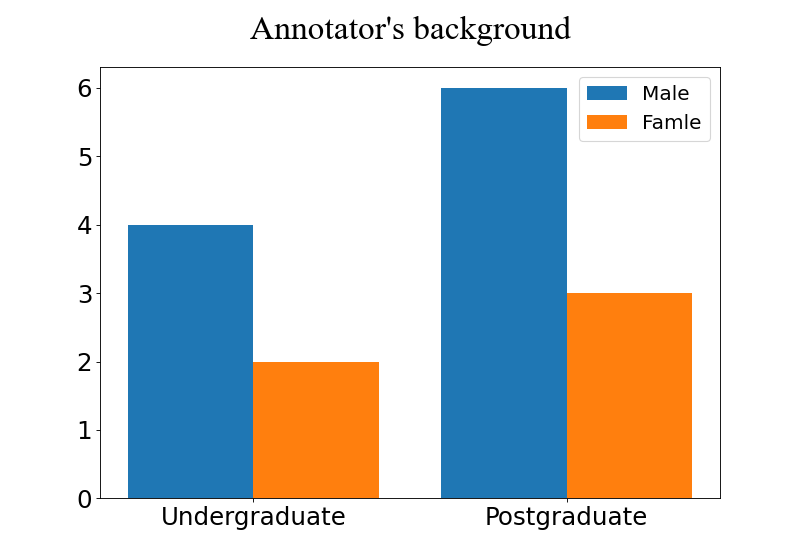}
    \caption{Annotator's detailed information}
    \label{fig:annotator detail}
\end{figure}

\subsection{Details of challenges}
\begin{figure}[h!]
    \flushleft
    \includegraphics[width=\linewidth]{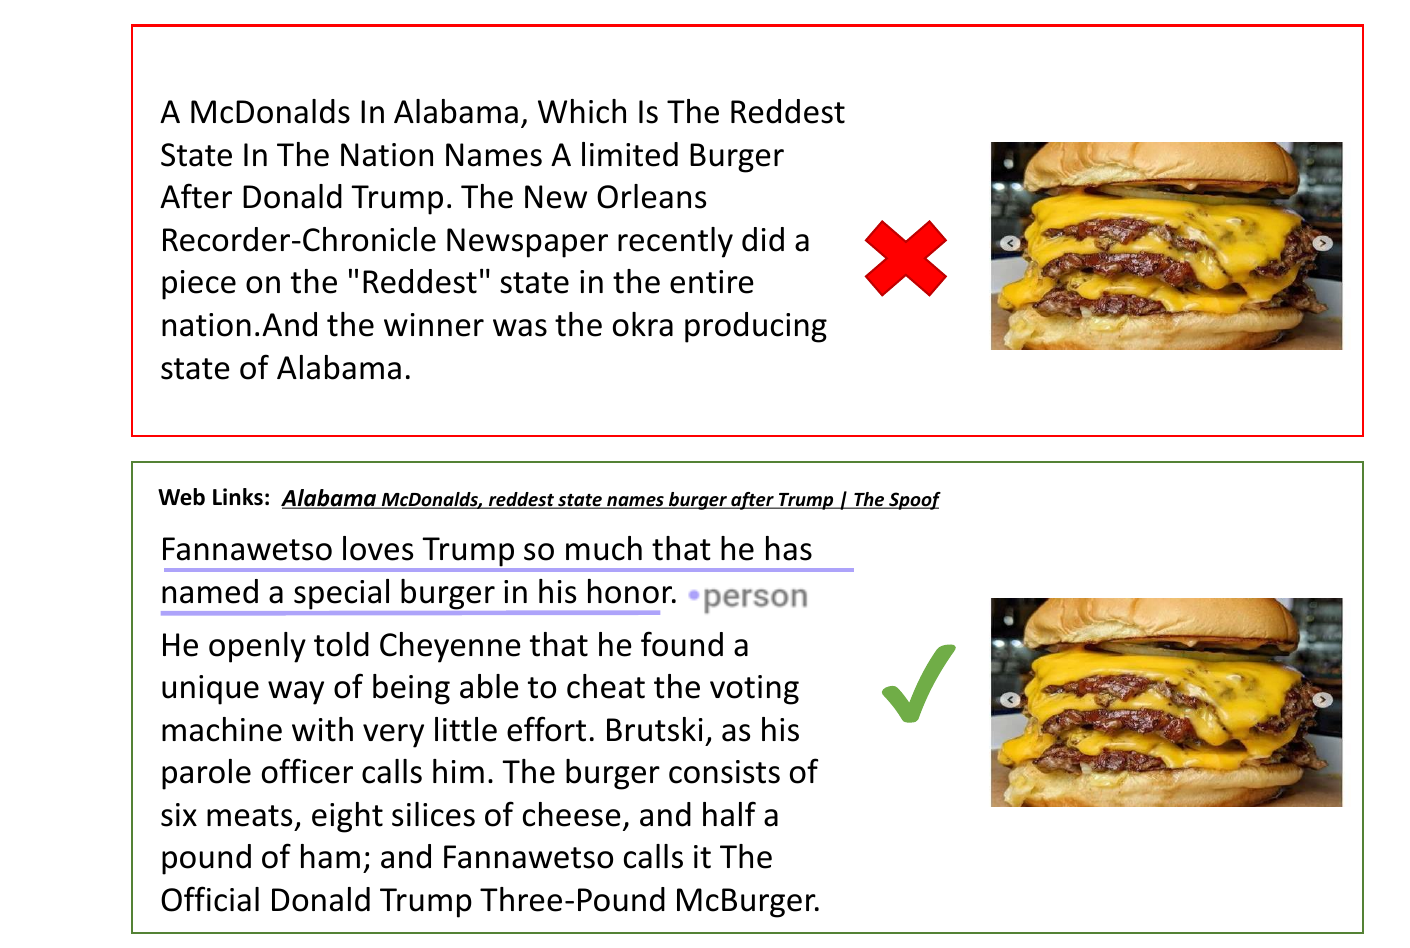}
    \caption{Detailed procedure to tackle the first annotation challenge in Section Annotation Process of the main paper}
    \label{fig:annotation detail}
\end{figure}

For the first annotation challenge ``Lacking explicit linguistic and visual markers in a sample'' that we have discussed in the Section Annotation Process of the main paper, we demonstrate how we address it in Figure \ref{fig:annotation detail}. As shown, the news title from a sarcastic web site ``The Onion'' says: \emph{A McDonalds in Alabama, which is the reddest state in the national names a limited burger after Donald Trump.}, accompanied with an abstract. An annotator may confuse about this piece of news by the news title and the picture, such as the relationship between "McDonalds" and  "Donald Trump" with the information provided. To assist the annotator to acquire more background knowledge, we provide a web link to such news, and then the annotator will read more detailed information and then manually select textual sarcastic clues to re-organize a sarcasm document that can be easily detected.  

Regarding the second annotation challenge ``Annotation variances caused by the subjective nature of perceiving sarcasm'' that we have discussed in Section Annotation Process of the main paper, we give Algorithm \ref{alg:thealg} to show the detailed procedure.

\begin{algorithm}[h!]
    \renewcommand{\algorithmicrequire}{\textbf{Input:}}
    \renewcommand{\algorithmicensure}{\textbf{Output:}}
\footnotesize
  \caption{Annotation scoring rules}
    \label{alg:thealg}
  {\textbf{Input parameters:} annots,datapool} \\
  {\textbf{Output:} {annot\_score},{sample\_score}} \; 
  \begin{algorithmic}
    \For{$round=1$ to $3$} 
      \Statex $dataset=random(datapool)$;
        \For{each $annot,sample$ in $annots,dataset$ }
        \Statex \quad$sample\_img, sample\_text$ $\leftarrow$ $sample$
        \Statex \quad img\_L\_round = annot($sample\_img$)
        \Statex \quad text\_L\_round = annot($sample\_text$)
      \If{$round$ > 1} 
        \For{$i=1$ to $round-1$}
            \Statex \quad\qquad ImgIOU = cal\_Img\_IOU(img\_L\_round-1,img\_L\_round)
            \Statex \quad\qquad TextIOU = cal\_Text\_IOU(text\_L\_round-1,text\_L\_round)
            \EndFor
            \Statex annot\_score += (imgIOU + TextIOU) 
            \Statex sample\_confidence += (imgIOU + TextIOU) 
      \EndIf
      \EndFor
      \EndFor
   \end{algorithmic}
\end{algorithm}

\subsection{Annotation platform}
We leverage an opensource doccano platform \cite{doccano} for textual and visual annotations.
Figure \ref{fig:Annotation platform} shows the website interface of annotations. 
The picture at the top is the interface of image annotations, where annotators are able to choose the sarcastic clue's type buttons and frame the sarcastic clues with bounding boxes.
The picture at the bottom of Figure \ref{fig:Annotation platform} is the interface for textual annotations, where annotators are able to mark the sarcastic clues. Note that, if the news is free of sarcasm, annotators just need to skip the news without any operations. 
\begin{figure*}[h!]
	\centering
        \includegraphics[scale=0.45]{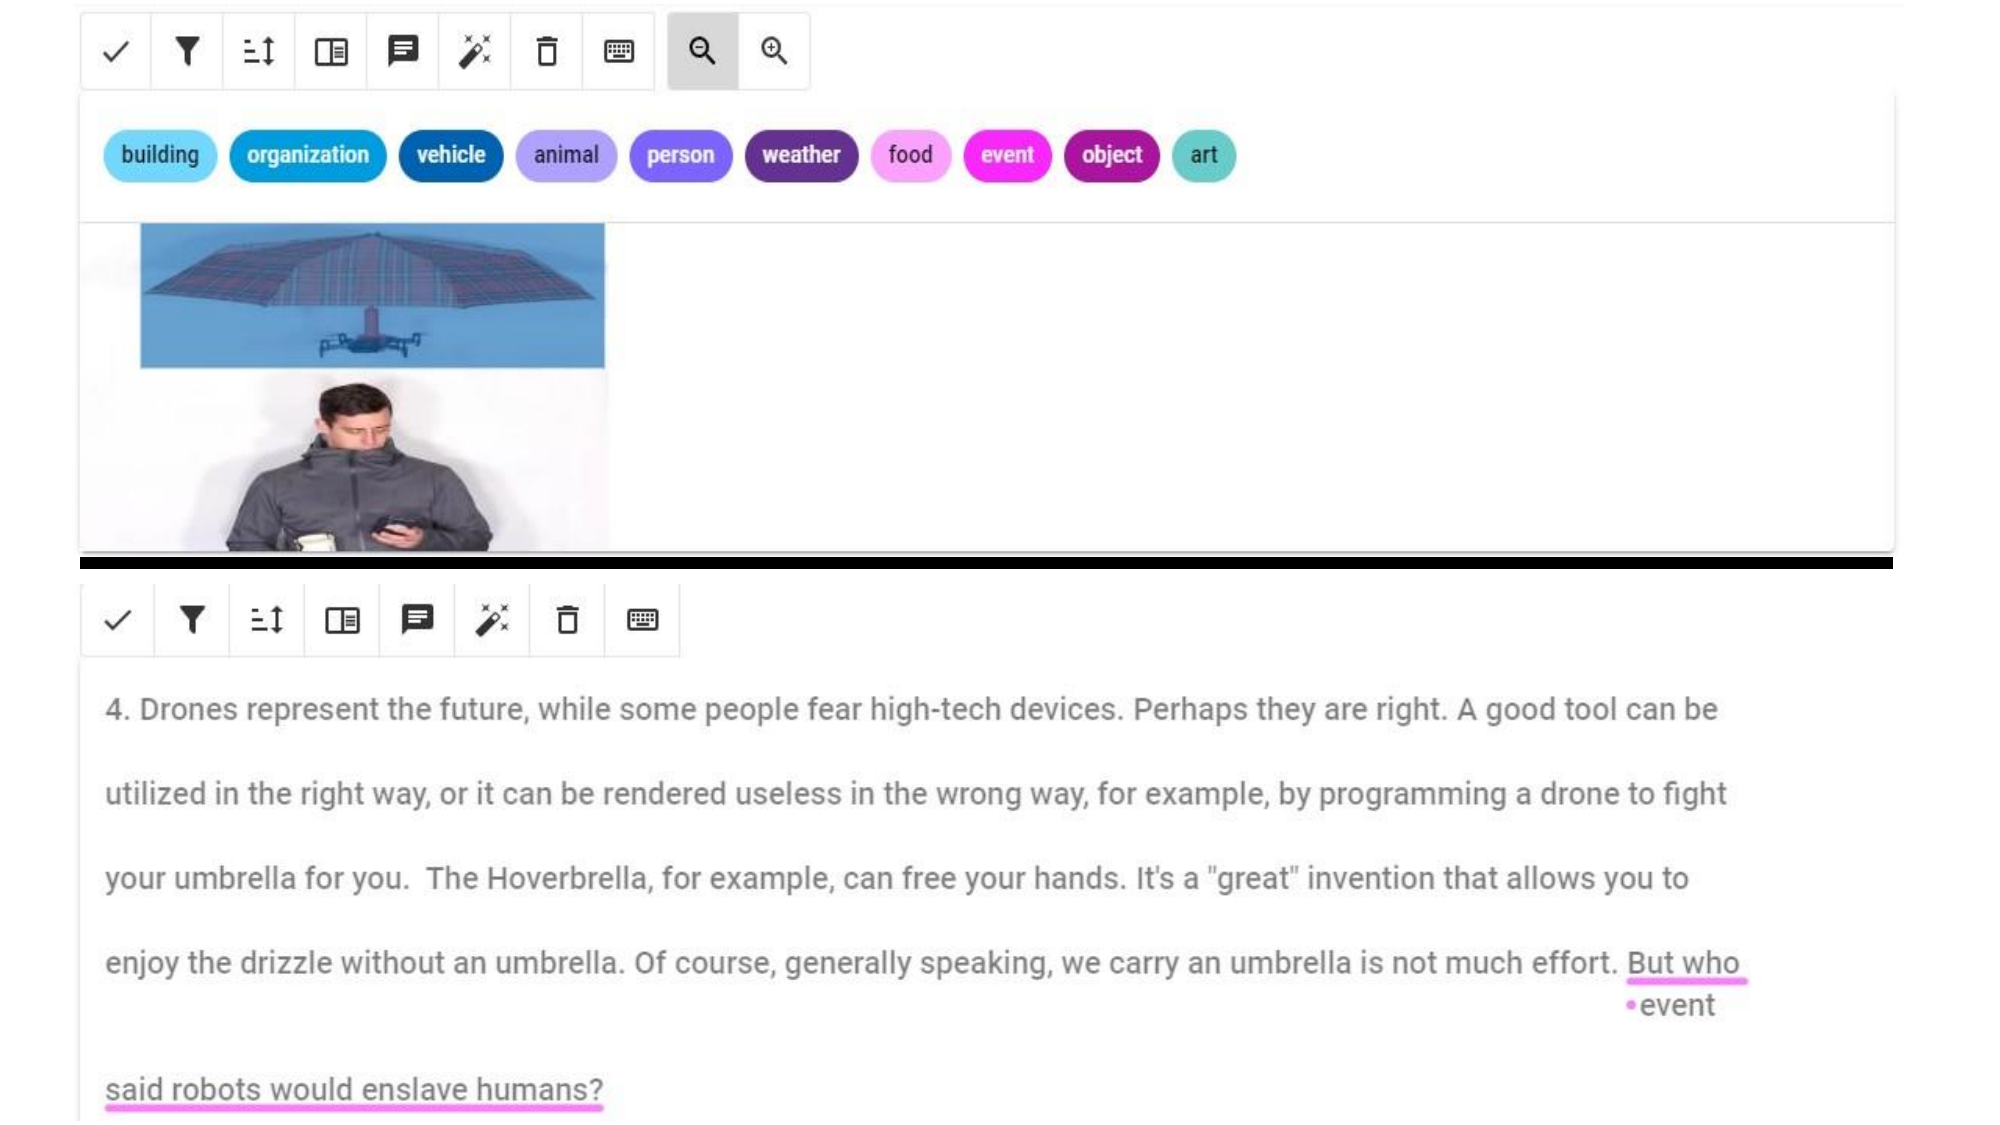}
	\caption{\textbf{Annotation platform.} The interface at the top shows the annotation process for the visual sarcastic clues, and the interface at the bottom shows the annotation process for textual sarcastic ones.}
        \label{fig:Annotation platform}
\end{figure*}
\subsection{Data Augmentation}\label{Appedix: Data Augmentation}
We used GPT-3.5 to expand the text part, and the process can be seen in Figure \ref{fig:GPT_augmentation}. Each text is expanded 5 times, while the image part remains the same, because the text is of high quality, GPT-3.5 can be expanded by adding details that do not affect the body of the event, while in the expansion we ask GPT-3.5 to replace as much sensitive information as possible.
\begin{figure*}[h!]
    \includegraphics[width=\linewidth]{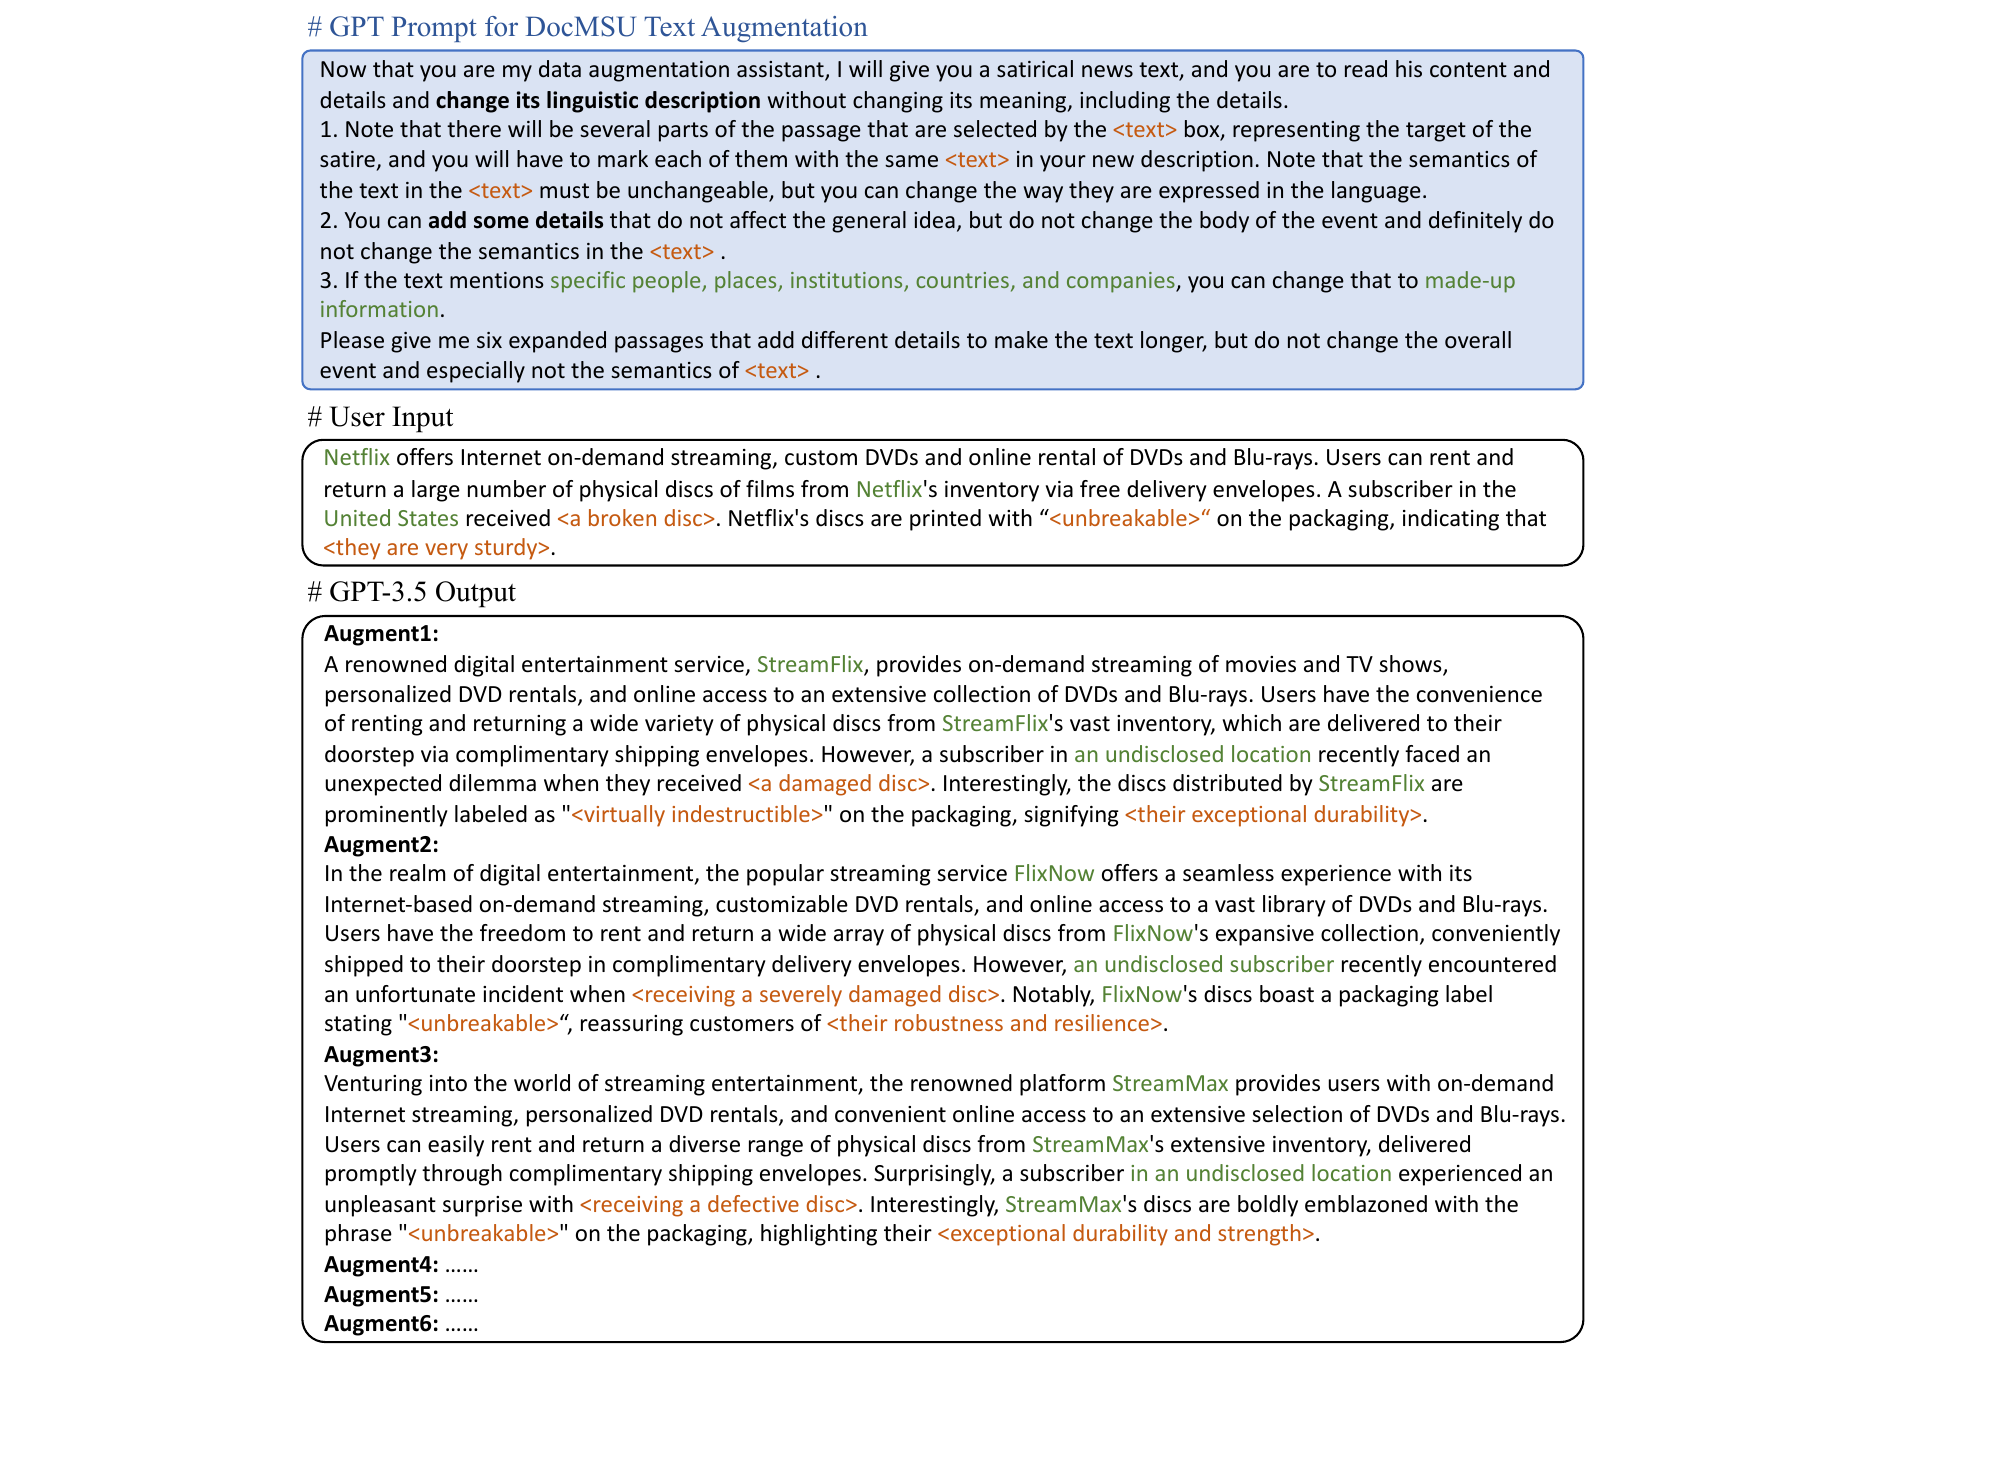}
    \caption{GPT-3.5 augmentation Process}
    \label{fig:GPT_augmentation}
\end{figure*}

\subsection{Dataset examples}\label{Appedix: Dataset examples}
This section shows some more data samples selected from our benchmark. As Figure \ref{fig:exp3} shows, in news a) "Back-to-school" is associated with learning and education, but in this case it is associated with alcoholic products, suggesting a celebration of students leaving to relax and enjoy life, and the irony of parents celebrating the departure of their children in contrast to the idea of true family reunion and care.\\In b), the vehicle was involved in an accident due to speeding and hit the warning sign. The contrast between the damaged vehicle scenario and the reminder sign can be interpreted as a sarcastic comment on the owner's driving ability, perhaps also implying that the use of the reminder sign was unreasonable and failed to remind the driver to drive carefully. \\In c), the health inspection report pictured here shows that the restaurant received an "A" rating, meaning it has excellent sanitation. However, the presence of a cockroach next to the report suggests that the restaurant actually has serious hygiene problems, a news clip that satirizes the reliability and accuracy of the rating system. \\ In d), the name of the restaurant next to SUBWAY in the picture is "fresh", which is very similar to SUBWAY's slogan "eat fresh". The irony of the news is that SUBWAY's slogan seems to suggest that customers should eat at a competitor's restaurant.

\begin{figure}[h!]
    \centering
    \includegraphics[width=1\linewidth]{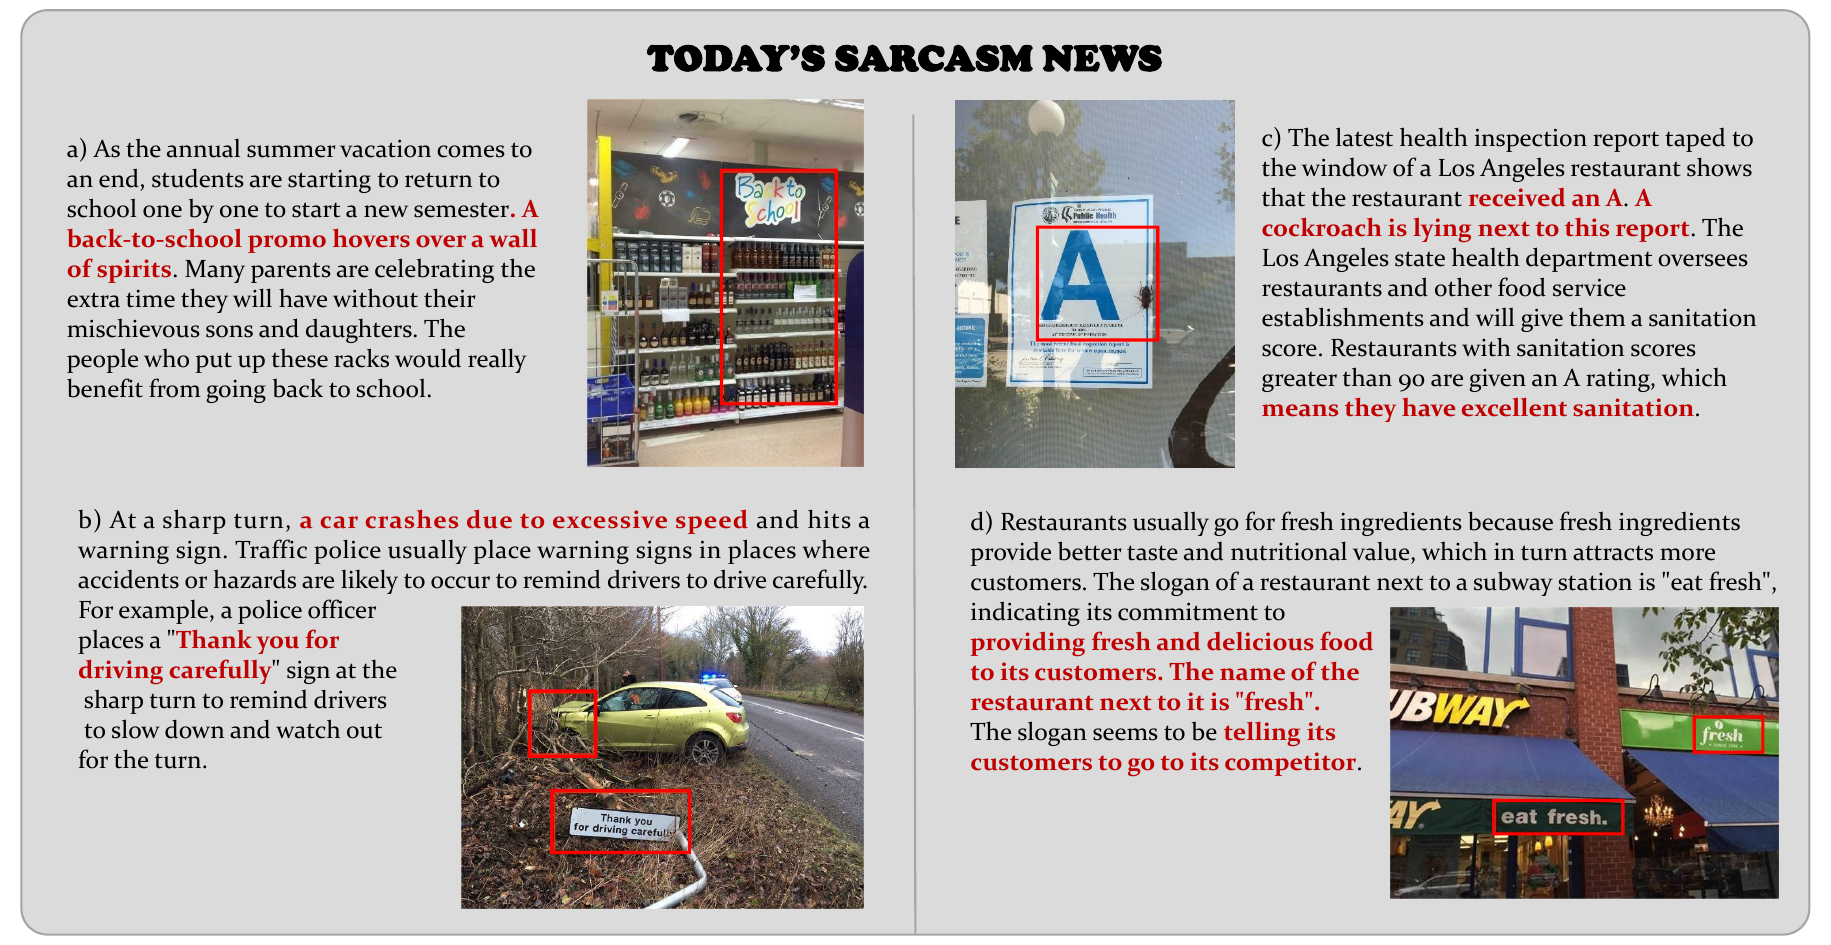}
    \caption{Four samples selected from our dataset}
    \label{fig:exp3}

\end{figure}

\section{Implementation Details and Settings}\label{Appedix: Implementation Details and Settings}
\label{sec:appendix}
% Please add the following required packages to your document preamble:
% \usepackage{multirow}
\begin{table}[h!]
\resizebox{0.98\columnwidth}{!}{
\setlength{\tabcolsep}{4pt} %% default is 6pt
\begin{tabular}{c|c|c} \bottomrule

\multirow{2}{*}{Resnet} & Conv          & {[}Kernel=3$\times$3,Padding=1,Stride=1{]} \\
                       & Activation    & ReLU                \\ \hline
\multirow{2}{*}{Proj}  & Conv          & {[}Kernel=4$\times$4,Padding=0,Stride=4{]} \\
                       & Normalization & LayerNorm           \\ \hline
\multirow{2}{*}{LM}    & Bert          & base                \\
                       & FC            & {[}Dim=768$\times$96{]}     \\ \hline
\end{tabular}}
\caption{Architecture of the proposed model}
\label{tab:architecture}
\end{table}
\noindent Table~\ref{tab:architecture} illustrates the architecture of our model. Specifically, for the image encoder, we simplified ResNet to a series of layers, each of which involves $3$ convolution kernels and an activation function. For each convolution layer, we set the kernel size, padding size, and stride as $3 \times 3$, $1$, and $1$, respectively. By doing so, we are able to keep the original resolution of images, facilitating pixel-level fusion with long text. The projection layer involves a convolution layer and a normalization layer, where the kernel size and the stride as $4 \times 4$ and $4$ respectively. In this way, we are able to generate the representations of each small patch of the image, and a patch contains $16$ pixels. For the document encoder, we leverage BERT-base to generate the contextualized representations of each word in the document, and then apply a fully connected layer (FC) to perform the transformation. We set the size of FC as [$768 \times 96$].
\section{Analysis of Swin-Transformer under Different settings}\label{Appedix: Analysis of Swin-Transformer under Different settings}

\begin{table}[h!]
\resizebox{0.98\columnwidth}{!}{
\begin{tabular}{ccccc} \bottomrule
\multicolumn{4}{c}{Sarcasm Detection}                        \\ \midrule
Swin-Transformer & Accuracy$\uparrow$  & Precision$\uparrow$       & F1-score$\uparrow$    \\ \midrule
Tiny              &  60.18 &       55.21   &   50.37                       \\ \midrule
Small             &  70.01 &       60.28   &   53.33                     \\ \midrule
Base              &  74.83 &       67.57   &   61.51                     \\ \bottomrule
\end{tabular}}
\caption{Different settings of Swin-Transformer}
\label{tab:settings}
\end{table}

\begin{table}[h!]
\resizebox{0.98\columnwidth}{!}{
\begin{tabular}{ccccc} \bottomrule
\multicolumn{5}{c}{Sarcasm Localization}                        \\ \midrule
Swin-Transformer & AP$_{50}$$\uparrow$  & F1$_{50}$$\uparrow$       & AP$_{60}$$\uparrow$    & F1$_{60}$$\uparrow$ \\ \midrule
Tiny              &  21.78 &       21.63   &   6.13   &     6.10                     \\ \midrule
Small             &  16.21 &       16.17   &   2.94   &     2.94                    \\ \midrule
Base              &  15.90 &       15.85   &   3.26   &     3.25                    \\ \bottomrule
\end{tabular}}
\caption{Different settings of Swin-Transformer}
\label{tab:settings}
\end{table}
In this section, we provide a more detailed description of the Swin-Transformer in experiments. We evaluate the baseline Swin-Transformer's performance under three settings including $Tiny$, $Small$ and $Base$. The experimental results in Table \ref{tab:settings} show that the Swin-Transformer of $Tiny$ setting achieves the best performance among the three settings in visual sarcasm localization, while the $Base$ setting performs best for sarcasm detection. Therefore, we report the results of the above two settings for the baseline Swin-Transformer. For fair comparisons, we also use the above two settings of Swin-Transformer as the backbone of our approach. The results show that our method achieves nearly $14$ points higher AP$_{50}$ under the backbone configured with $Tiny$ for visual sarcasm localization, indicating the superiority of our method in capturing the nuanced sarcastic clues.

\section{Analysis of Image Encoder Under Different Settings}\label{Appedix: Analysis of Image Encoder Under Different Settings}
\begin{table}[h!]
\resizebox{1\columnwidth}{!}{
\begin{tabular}{ccccc} \bottomrule
\multicolumn{5}{c}{Sarcasm Localization}                        \\ \midrule
Layers of Resnet & AP$_{50}$$\uparrow$  & F1$_{50}$$\uparrow$       & AP$_{60}$$\uparrow$    & F1$_{60}$$\uparrow$ \\ \midrule
0                &        22.42       &     22.36   &        1.95        &     1.95 \\ \midrule
1                &        29.58       &     29.48   &        10.82       &    10.79  \\ \midrule
2                &        32.64       &     32.53   &        11.28       &    11.22  \\ \midrule
3                &        35.29       &     35.24   &        13.74       &    13.67  \\ \midrule
4                &        31.65       &     31.60   &        12.78       &    12.74  \\ \midrule
5                &        27.60       &     27.55   &         9.01       &     8.27  \\ \bottomrule
\end{tabular}}
\caption{Analysis of image encoder for visual sarcasm localization}
\label{tab:blocks-in-image}
\end{table}
\begin{table}[h!]
\resizebox{1\columnwidth}{!}{
\begin{tabular}{ccccc} \bottomrule
\multicolumn{5}{c}{Sarcasm Localization}                        \\ \midrule
Layers of Resnet & EM$_{50}$$\uparrow$  & EM$_{70}$$\uparrow$       & EM$\uparrow$    &  BitError$\downarrow$ \\ \midrule
0                &     50.21          &      39.11  &        37.67       &    17.05 \\ \midrule
1                &     50.29          &      41.33  &        39.21       &    17.69   \\ \midrule
2                &     51.37          &      41.51  &        39.29       &    16.56  \\ \midrule
3                &     52.19          &      43.88  &        39.66       &    17.67  \\ \midrule
4                &     52.02          &      40.85  &        39.02       &    16.56 \\ \midrule
5                &     50.71          &      41.06  &        38.33       &    16.66  \\ \bottomrule
\end{tabular}
}
\caption{Analysis of image encoder for textual sarcasm localization}
\label{tab:blocks in text}
\end{table}
We use ResNet as our image encoder and simplify the networks to several layers, each of which contains $3$ convolution kernels and a RELU function for the image encoder. We further analyze the performance of our method for visual sarcasm localization, under the different number of encoder layers. In terms of AP$_{50}$, the results in Table \ref{tab:blocks-in-image} show that the performance consistently increases from $22.42$ to $35.29$ when the number of layers is increased from $0$ to $3$. It reaches the peak under the $3$ layers and then sharply decreases if we continue to stack more layers for the encoder. These results suggest that we should have a good tradeoff between the complexity of the image encoder and the performance of sarcasm localization.

%Table \ref{tab:blocks-in-image} reports the performance of visual sarcasm localization. 
%It could be concluded that the performance of the model with Resnet is significantly better than that of the model without Resnet, and the model gets the best performance when the number of layers is $3$.
%Table \ref{tab:blocks in text} reports the performance in the task of sarcasm localization in text. 
%It could be seen that the model gets the best performance when the number of layers is $3$, which confirms that the fine-grained features in image 
%are effective for sarcasm localization in texts as well.
\section{Case Study}\label{Appedix: Case Study}
\begin{figure}[ht!]
    \includegraphics[width=1\linewidth]{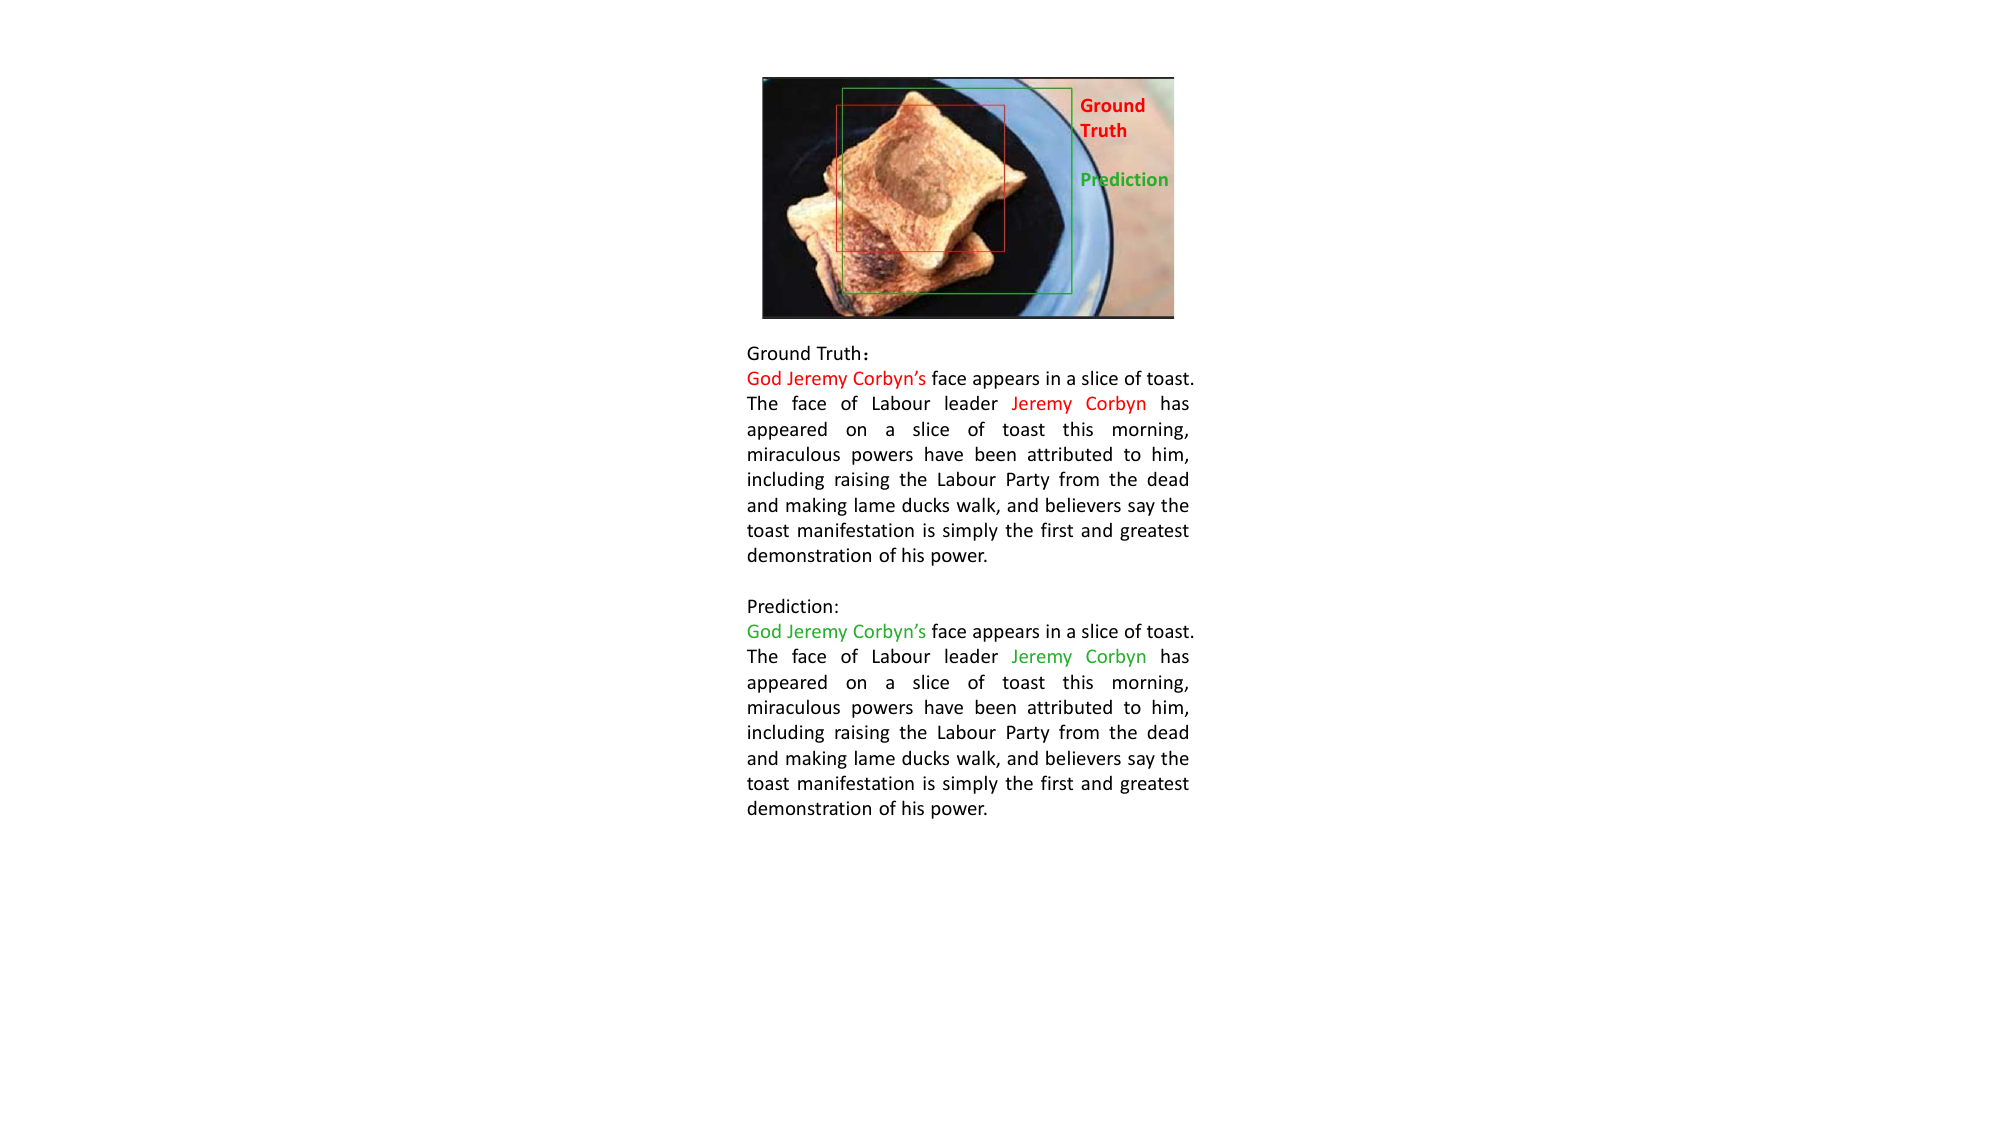}
    \caption{A case study}
    \label{fig:case study}
    \vspace{-4mm}
\end{figure}

We give a case in Figure \ref{fig:case study} to visually show the effectiveness of our method in identifying the sarcastic clues. This case mocks that a political leader hopes that he can be treated as God. The ground truth of the visual sarcastic clue is the bounding box highlighted in red color, and the textual ones are concealed in $5$ words including ```God Jeremy Corbyn's'' and ``Jeremy Corbyn'' in the document of $61$ tokens. For this case, our method is able to accurately localize the visual and textual clues, showing the superiority of our model for the challenging MSU task.  

%The targeting news contains $61$ words in the document, and our model is able to accurately localize the sarcastic clues in the document, which are only $5$ words and sparsely distributed. In the task of localization in images, our model is able to frame the sarcastic clues in image. This case verifies the fine-grained features' superiority in the task of localization in both document and image. 

\section{Tests on LLMs}\label{Appedix: Tests on LLMs}
\begin{figure*}[h!]
    \includegraphics[width=0.97\linewidth]{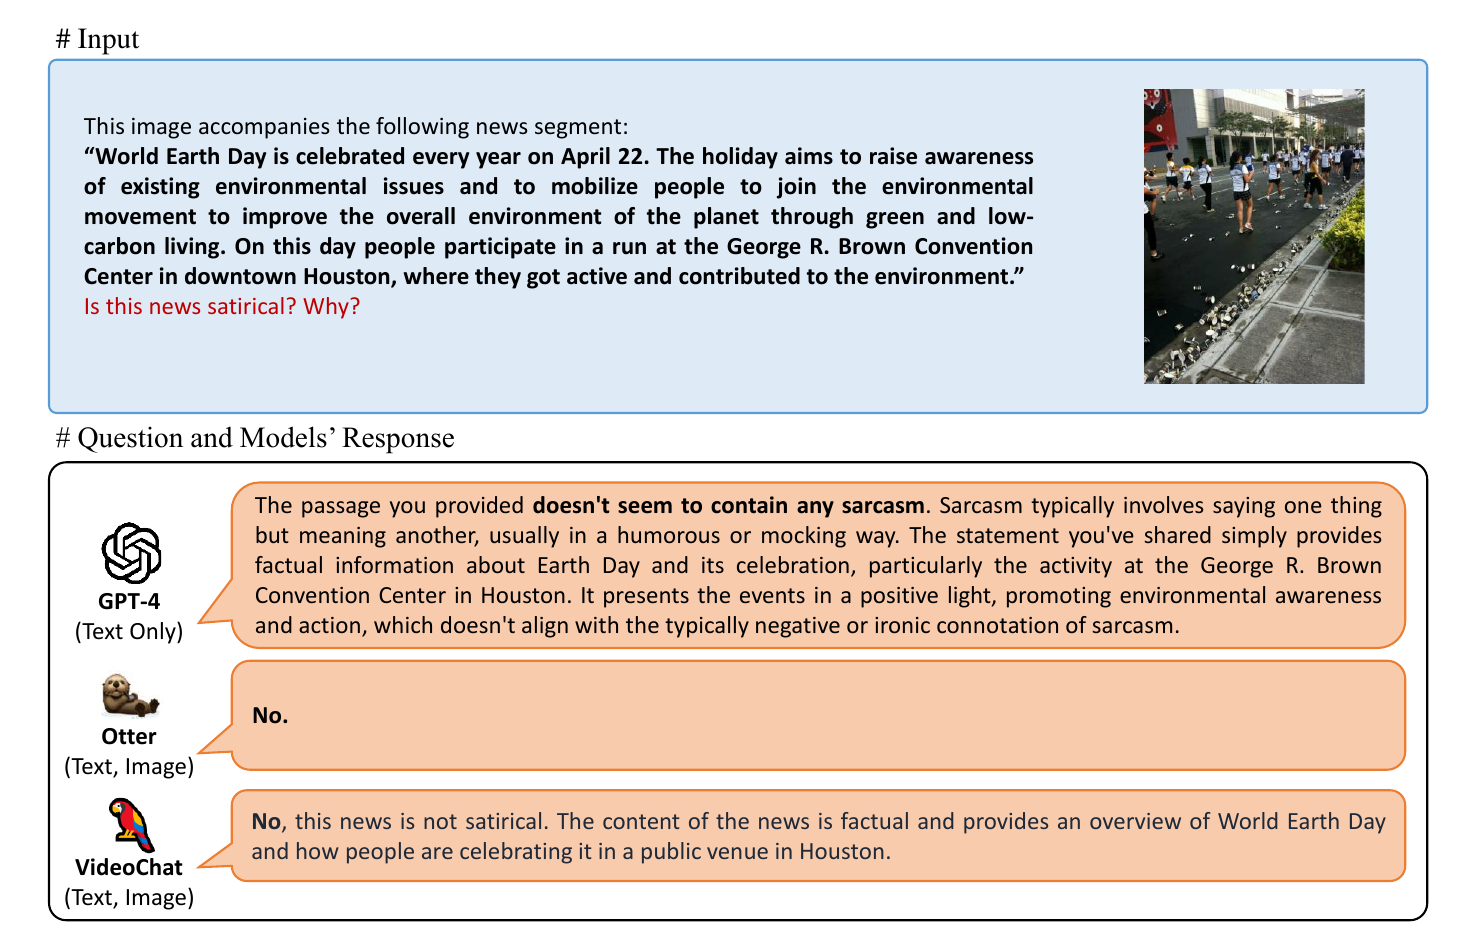}
    \caption{LLMs response}
    \label{fig:tests on LLMS}
 \vspace{-4mm}
\end{figure*}
We tested on three LLMs, and the results of one of the tests are given in Figure \ref{fig:tests on LLMS}, from which we can see that GPT-4 failed to recognize the irony of the text without inputting the image, while Otter and VideoChat failed to compare the information about the paper cup on the ground and the environmental activities in the text and recognize the irony after inputting the image text pairs.

\section{Limitations}\label{Appedix: Limitations}
\textbf{Benchmark:} Previous studies \cite{Rockwell,talkischeap} show that the way of irony expression can vary across social cultural backgrounds. Further, existing works also discussed that females tend to have a more self-deprecating attitude than males when using sarcastic expressions \cite{Sogancioglu2022TheEO}. We collect data from famous American websites without considering the above impacts on the sarcasm understanding \cite{Dress}, though our DocMSU already covers $9$ hot topics, each of which includes $10$ target types in the news field.\\  
\textbf{Model:} Generative methods have shown their promise in multimodal understanding. Along this line, we would like to further investigate how our text and image encoder can be extended to a generative method to better fuse the fine-grained multimodal information. We are also interested in improving Swin-Transformer, the backbone of our model, by exploring a multi-stage mechanism based on the previously proposed FPN \cite{8099589} and PA-NET\cite{liu2018path}. Such design has been discussed in the field of semantic segmentation \cite{7803544}.

\bibliographystyle{plain}%
\bibliography{sup}
\end{document}
